# Supplementary material for: Symmetric Gapped States and Symmetry-Enforced Gaplessness in 3-dimensions
Source: arXiv:2602.12335 source file (2026-10-12)
Supplement: Supplementary file 1 [file supplementary.tex]

\documentclass[aps,pra,amsmath,amssymb, notitlepage, 
twocolumn,
nofootinbib,
superscriptaddress,
longbibliography,10pt
]{revtex4-1}
\usepackage{amsmath}
\usepackage{amsthm}
\numberwithin{equation}{section}
\usepackage{tabularx,graphicx}
\usepackage{epstopdf}
\usepackage{makecell}
\usepackage{latexsym}
\usepackage[dvipsnames]{xcolor}
\usepackage{colortbl}
\usepackage{psfrag}
\usepackage{bbm}
\usepackage{bm}
\usepackage{titlesec}
\usepackage{dsfont}
\usepackage{feynmp}
\usepackage{slashed}
\usepackage{multirow}
\usepackage{url}

\newcommand{\beq}{\begin{eqnarray}}
	\newcommand{\eeq}{\end{eqnarray}}

\newcommand{\bsp}{\begin{aligned}}
	\newcommand{\esp}{\end{aligned}}

\definecolor{darkblue}{rgb}{0.,0.,0.4}
\definecolor{darkred}{rgb}{0.5,0.,0.}
\definecolor{BlueViolet}{RGB}{138,43,226}
\definecolor{SkyBlue}{RGB}{30,144,255}
\definecolor{DarkGreen}{RGB}{0,100,0}

\usepackage{mathtools}

\usepackage{tikz-cd}
\usepackage{booktabs}

%\usepackage[unicode=true,pdfusetitle,
%   bookmarks=true, 
%   bookmarksnumbered=false, 
%   bookmarksopen=false,
%   breaklinks=false, 
%   pdfborder={0 0 1}, 
%   backref=false, 
%   colorlinks=true, linkcolor=darkblue, citecolor=blue, urlcolor=darkred]{hyperref}
%\hypersetup{pdfauthor={Liujun}}
\usepackage{hyperref}
\usepackage[capitalize, noabbrev]{cleveref} % TODO: package options

\usepackage[normalem]{ulem}

%%%% Commenting & change tracking

\usepackage{mathrsfs}
\usepackage{comment}

\newcommand{\Z}{\mathbb{Z}}

\usepackage{pst-all}
\usepackage{leftidx}
\usepackage[off]{auto-pst-pdf} %%%Speeds up compilation but does not compile any new pstricks figures or recompile old ones.
\usepackage{yfonts}
%\makeatletter
%%%%%%%%%%%%%%%%%%%%%%%%%%%%%% LyX specific LaTeX commands.
%% Because html converters don't know tabularnewline

%%%%%%%%%%%%%%%%%%%%%%%%%%%%%% User specified LaTeX commands.

\usepackage{svg}

%%%%%%%%%%%%%%%%%%%%%%%%%%%%%%%%%%% Other stuff imported from CMP template

\newtheorem{lem}{Lemma}

\newtheorem*{thm*}{Theorem}

\theoremstyle{definition}

\theoremstyle{remark}

\crefname{cor}{Corollary}{Corollaries}

\crefname{thm}{Theorem}{Theorems}
\Crefname{thm}{Theorem}{Theorems}
\crefname{prop}{Proposition}{Propositions}
\crefname{lem}{Lemma}{Lemmas}
\crefname{defn}{Definition}{Definitions}

\hypersetup{
    colorlinks=true,
    linkcolor=darkblue,
    citecolor=blue,
    urlcolor=darkred
}
\usetikzlibrary{calc}
%\usetikzlibrary{external}
%\tikzexternalize

%\renewcommand{\thesubsection}{\arabic{subsection}}

\usepackage[mathscr]{eucal}
\makeatletter
\def\instring#1#2{TT\fi\begingroup
  \edef\x{\endgroup\noexpand\in@{#1}{#2}}\x\ifin@}
\def\isuppercase#1{%
  \instring{#1}{ABCDEFGHIJKLMNOPQRSTUVWXYZ}%
}%
\newcommand{\C@lIfUpper}[1]{
 \if\isuppercase{#1}\mathscr{#1}%
 \else #1%
 \fi
}
\newcommand{\cat}[1]{\mathit{\@tfor\next:=#1\do{\C@lIfUpper{\next}}}}
\makeatother

\usepackage{xparse}

\newcommand{\U}{\mathrm U}

\newcommand{\bl}{\text{--}}

\newcommand{\SH}{\mathrm{SH}}

\newcommand{\tVect}{\mathbf{2Vect}}
\newcommand{\tsVect}{\mathbf{2sVect}}

\newcommand{\fB}{\mathfrak B}

% https://tex.stackexchange.com/questions/456307/invalid-use-of-intertext-in-aligned
\newcommand{\alignedintertext}[1]{%
  \noalign{%
    \vskip\belowdisplayshortskip
    \vtop{\hsize=0.75\linewidth#1\par
    \expandafter}%
    \expandafter\prevdepth\the\prevdepth
  }%
}

%%%%Email
\newcommand\MAILTO[1]{\href{mailto:#1}{\nolinkurl{#1}}}

% Short exact sequences: write
% \shortexact[f][g]{A}{B}{C}, for:
%
% f g
% 0 -> A -> B -> C -> 0,
% (or 1 -> A -> B -> C -> 1 with a star)
\DeclareDocumentCommand{\shortexact}{s O{} O{} mmmm}{
\IfBooleanTF{#1}{ % if star
\begin{tikzcd}[ampersand replacement=\&]
	{1} \& {#4} \& {#5} \& {#6} \& {1#7}
	\arrow[from=1-1, to=1-2]
	\arrow["#2", from=1-2, to=1-3]
	\arrow["#3", from=1-3, to=1-4]
	\arrow[from=1-4, to=1-5]
\end{tikzcd}
}{ % no star
\begin{tikzcd}[ampersand replacement=\&]
	{0} \& {#4} \& {#5} \& {#6} \& {0#7}
	\arrow[from=1-1, to=1-2]
	\arrow["#2", from=1-2, to=1-3]
	\arrow["#3", from=1-3, to=1-4]
	\arrow[from=1-4, to=1-5]
\end{tikzcd}
}}

% tikz utility to draw the A(1)-module M_0.
% first two arguments are the x- and y-coords; the third is the name of the lowest-degree point
%\newcommand{\Mzero}[3]{
%	\tikzpt{#1}{#2}{#3}{};
%	\foreach \y in {2, 3, 5} {
%		\tikzpt{#1}{#2 + \y}{}{};
%	}
%	\sqone(#1, #2 + 2);
%	\sqtwoL(#1, #2);
%	\sqtwoL(#1, #2 + 3);
%}

% TODO: WIP footnote formatting
% the problem is something to do with RevTeX -- if you copy in the standard defn of \@makefntext, the margin error persists
%\makeatletter
%\renewcommand\@makefntext[1]{%
%    \parindent 1em%
%    \noindent
%    \hb@xt@1.8em{\hss\@makefnmark}#1}
%\long\def\@makefntext#1{%
%\def\baselinestretch{1}%
%\leftskip1em%
%\parindent1em%
%\noindent
%\nobreak%
%\hskip-\leftskip
%\hb@xt@\leftskip{%
%\hss\@makefnmark\ %
%}%
%#1%
%\par
%}%
%\makeatother

% shortcut for drawing an h_0-tower in an Adams spectral sequence chart

\usepackage{xspace}

% make cleveref use the Oxford comma:
% see https://tex.stackexchange.com/questions/161338

% source: https://tex.stackexchange.com/a/596811/55879
% ********************* added<<<<<<<<<<<<<<<<<<<<
\makeatletter 
    
\renewcommand\onecolumngrid{% <<<<<<
\do@columngrid{one}{\@ne}%
\def\set@footnotewidth{\onecolumngrid}% <<<<<<<<<<<<<<<<
\def\footnoterule{\kern-6pt\hrule width 1.5in\kern6pt}%
}

\renewcommand\twocolumngrid{% <<<<<<
        \def\footnoterule{% restore rule
        \dimen@\skip\footins\divide\dimen@\thr@@
        \kern-\dimen@\hrule width.5in\kern\dimen@}
        \do@columngrid{mlt}{\tw@}
}%

\makeatother

% I am confused as to why this works. -AD
\makeatletter
\renewcommand{\p@subsection}{}
\makeatother

%%  *********************************************** 

\setcounter{tocdepth}{-1}

\begin{document}

\count\footins = 1000

\title{Supplemental Material for ``Symmetric Gapped States and Symmetry-Enforced Gaplessness in 3-dimension''}

\author{Arun Debray}
\affiliation{Department of Mathematics, University of Kentucky, 719 Patterson Office Tower, Lexington, KY 40506-0027}
\email{a.debray@uky.edu}

\author{Matthew Yu}
\affiliation{Mathematical Institute, University of Oxford,  Woodstock Road, Oxford, UK}
\email{yumatthew70@gmail.com}

\author{Weicheng Ye}
\affiliation{Department of Physics and Astronomy, and Stewart Blusson Quantum Matter Institute, University of British Columbia, Vancouver, BC, Canada V6T 1Z1}
\email{victoryeofphysics@gmail.com}

\maketitle

In this supplementary material, we provide an overview of supercohomology and sketch the proofs of Theorems 1 and 2 in the main text. This exposition is intended for a physics audience; full mathematical details are provided in Ref.~\cite{Debray:2025kfg}.

\section{Supercohomology}\label{appendix:supercoh}

We approach the definition of supercohomology through the lens of fermionic symmetry-protected topological (SPT) states~\cite{Kit13,Kit15,PhysRevX.10.031055} in the end matter. In the absence of symmetry, fermions admit nontrivial gapped phases known as \emph{invertible states}. These are short-range entangled quantum states that possess an inverse, such that stacking the state with its inverse yields a trivial gapped vacuum. The classification of fermionic SPT phases is built upon these invertible states using the decorated domain wall picture~\cite{Wang:2017moj,PhysRevX.10.031055}, which organizes the classification data into four distinct layers: $p+ip$ layer, Majorana layer, Gu-Wen layer, and the Dijkgraaf-Witten layer. If we restrict our attention to the subset of the full classification that ignores the decoration of $p+ip$ invertible states in 2 spatial dimensions, we recover the data described by supercohomology. From this definition, it is clear that supercohomology serves as an approximation of the full classification of fermionic SPT states or fermionic 't Hooft anomalies by anomaly inflow. 

From the point of view of category theory, we can also organize these invertible states, aside from the $p+ip$ layer, as the Picard 2-groupoid $\tsVect^\times$ comprising of Morita-invertible complex superalgebras, super Morita equivalences, and intertwiners. Within this framework, the only nontrivial object (up to Morita equivalence) is the Clifford algebra $\mathrm{Cl}(1)$. The morphisms and 2-morphisms in this category correspond to bimodules and bimodule maps, respectively. By computing the homotopy groups of these constituents, one recovers the layered structure of supercohomology: a 2-form part $\Z_2$ corresponding to the Majorana layer, a 1-form part $\Z_2$ corresponding to the Gu-Wen layer, and a 0-form part $\U(1)$ corresponding to the Dijkgraaf-Witten layer. These components assemble into a nontrivial 3-group~\cite{Gaiotto:2017zba,Yu:2020twi}.

Expressing supercohomology from the perspective of $\tsVect^\times$ naturally connects the fusion 2-category description of fermionic topological orders in a very convenient way. In particular, topological orders in 3 spatial dimensions should have operators that together form a braided fusion 2-category. In the bosonic setting, the corresponding braided fusion 2-category is \emph{non-degenerate}, which means that any operator must braid non-trivially with some operator physically. Mathematically, the non-degeneracy is translated into the fact that the \emph{sylleptic center} of the braided fusion 2-category for bosonic systems is $\tVect$.  In the fermionic setting, we can have a local fermion that braids trivially with all other operators. Therefore, the {sylleptic center} of the braided fusion 2-category for fermionic systems is indeed $\tsVect$, and these braided fusion 2-categories are called non-degenerate fermionic braided fusion 2-categories.

To enrich a nondegenerate fermionic braided fusion 2-category $\fB$ with a $G$ symmetry, we need to introduce $G$-defects that permute the theory's operators. Mathematically, it means that the symmetry action invokes a nontrivial map from the symmetry group $G$ to the Picard groupoid of $\fB$, and an obstruction to this map is captured by a 5-groupoid that contains $\tsVect^\times$. Consequently, this strongly suggests that anomalies for fermionic topological orders take values in supercohomology. The mathematical details of these facts, including the interpretation of various pieces in the Wang--Wen--Witten construction from the point of view of category theory, are presented in Refs.~\cite{Decoppet:2025eic,D8,D11,Debray:2025kfg}.

\section{Theorem 1}
\label{appendix:thm3}

We now give a summary of our proof of Theorem 1.
Let $G$ be a finite group and $\alpha\in\SH^n(G)$ with $n\geq 5$. The formal statement of the result is that there is an algorithmic construction of a finite group $\widetilde G$ and a map $\rho\colon \widetilde G\to G$ such that \begin{equation}
    \rho^*(\alpha) = 0\in \SH^n(\widetilde G).
\end{equation}
From this, we naturally get a short exact sequence of groups
\begin{equation}
1 \rightarrow K \rightarrow \widetilde{G}\rightarrow G \rightarrow 1,
\end{equation}
such that after gauging $K$ symmetry of a $\widetilde{G}$-symmetric state we get a $K$-gauge theory with the prescribed anomaly $\alpha$. 

The proof of this result proceeds by trivializing one layer of the anomaly at a time.  Namely, we find a group $G_1\rightarrow G$ such that the Majorana layer is trivialized, then we find a group $G_2\rightarrow G_1$ such that the Gu--Wen layer is trivialized, and finally we find a group $\widetilde{G}\rightarrow G_2$ such that the bosonic layer is also trivialized. 

We employ the following lemma to guarantee that it is possible to trivialize each layer: 
\begin{lem}\label{thm:folk}
    Let $G$ be a finite group, $M$ be a $\Z[G]$-module, $n\ge 3$, and $\alpha\in H^n(G; M)$. Then there is an algorithmic construction of a finite group $\widetilde G$ and a homomorphism $\rho\colon \widetilde G\to G$ such that $\rho^*(\alpha) = 0$.
\end{lem}

We finish the proof of the theorem by analyzing how the full (supercohomology) anomaly can be mapped to each of its layers, which are themselves valued in ordinary cohomology.  We construct  a map
\begin{equation}
    (\bl)_{\mathrm{Maj}}\colon \SH^n(G) \longrightarrow H^{n-2}(G; \Z/2),
\end{equation}
that sends a class $\alpha$ to its {Majorana layer} $\alpha_{\mathrm{Maj}}$. Using \Cref{thm:folk} we find an extension $G_1\rightarrow G$ that trivializes the Majorana layer. We repeat the process, now replacing supercohomology with reduced supercohomolgy composed with the information from two layers instead of three \cite{Wang:2017moj}. Again invoking \Cref{thm:folk}, we are able to construct a group $G_2\rightarrow G$ such that pulling back the class in reduced supercohomology trivializes the Gu-Wen layer. This leaves only the bottom Dijkgraaf-Witten layer to trivialize, for which we again use \Cref{thm:folk}.

\section{Theorem 2}
\label{appendix:thm4}

We now give a summary of our proof of Theorem 2. As reviewed in the end matter, given a group $G$ and an element of the full 't Hooft anomaly $\alpha\in \mho^5(G)$, it has a natural projection into \begin{equation}
(\bl)_{p+ip}\colon \mho^5(G) \rightarrow H^2(G;\Z)\cong H^1(G;\U(1)).
\end{equation}
The image $\alpha_{p+ip}\in H^1(G;\U(1))$ characterizes the information regarding the decoration of the $p+ip$ layer. Moreover, it can be thought of as a map $\alpha_{p+ip}\colon G\rightarrow\U(1)$. It is known in Ref.~\cite{Hsi18} that given any element $\alpha_{p+ip}\in H^1(G;\U(1))$, it is impossible to trivialize this element by a short exact sequence 
\begin{equation}
1 \rightarrow K \rightarrow \widetilde{G}\rightarrow G \rightarrow 1,
\end{equation}
unlike what we have done for supercohomology. However, this simple argument is insufficient, as it is possible to construct anomalous topological orders using methods other than symmetry extension. We provide a rigorous proof that refines the approach taken in Ref.~\cite{CO2}. Specifically, we analyze the partition function on $K3 \times S^1$ by employing an algebraic-topological argument applicable to all symmetry groups. Unlike the original approach, our method does not rely on the Atiyah-Singer index theorem and is therefore generalizable to all fermionic systems (field theories). Following the analysis of the partition function on the K3 surface established in Ref.~\cite{CO2}, we complete the proof. 

The key lemma in our proof is as follows.
\begin{lem}\label{thm:folk2} 
    Let $G$ be a finite group, $\alpha\in \mho^5(G)$ a beyond-cohomology anomaly corresponding to an element $\alpha_{p+ip}\colon G\rightarrow\U(1)$. Consider the corresponding invertible field theory of $\alpha$. Its partition function on $\mathrm{K3}\times S^1_g$, where the subscript $g\in G$ denotes a nontrivial holonomy around $S^1$, is given by $\alpha_{p+ip}(g)\in \U(1)$.
\end{lem}

Our proof proceeds by a mathematically rigorous definition of ``compactification on the K3 surface''. The outcome of the compactification is an invertible field theory in one dimension, which is exactly characterized by $\alpha_{p+ip} \in \mho^1(G)$. Evaluating the partition function of $\alpha_{p+ip}$ on $S^1_g$ will then give the desired result.

The rest of the proof follows the analysis in Ref.~\cite{CO2}, and we briefly repeat it here for the reader's convenience. On the one hand, Lemma~\ref{thm:folk2} immediately suggests that for \emph{any} quantum theory in 3 spatial dimensions with anomaly $\alpha$, its partition function on K3 surface, i.e., $Z(\mathrm{K3})$, is acted upon nontrivially by elements $g\in G$. The only possibility is $Z(\mathrm{K3}) = 0$. On the other hand, a topological order is described by a (3+1)-dimensional topological quantum field theory (TQFT). The axioms of TQFTs guarantee that the partition function on K3 surface can never be zero. Therefore, the quantum theory in 3 spatial dimensions with anomaly $\alpha$ can never be a TQFT or a topological order.

\bibliography{reference}

\end{document}
